# Supplementary material for: Topological Hall Effect in Magnetic Topological Insulator Films
Source: arXiv:1809.02210 ancillary file (2018-09-06)
Supplement: Supplementary file 1 [file supplementary.pdf]

# Supplementary Materials for "Topological Hall Effect in Magnetic Topological Insulator Films"

Jian-Xiao Zhang,[1] Domenico Andreoli,[2] Jiadong Zang,[2] and Chao-Xing Liu[1]

[1] *Department of Physics, The Pennsylvania State University, University Park, Pennsylvania 16802-6300, USA*

[2] *Department of Physics, University of New Hampshire, Durham, New Hampshire 03824, USA*

## Appendix A: From 3D TI Hamiltonian to 2D thin film Hamiltonian

In this section, we follow the derivation in Ref. [1] to construct the Hamiltonian for the 2D topological insulator (TI) films. We start from the 4 band model [2] of 3D TI,

$$H_{3D}(\boldsymbol{k}) = \begin{pmatrix} M(\boldsymbol{k}) & 0 & A_1 k_z & A_2 k_- \\ 0 & M(\boldsymbol{k}) & A_2 k_+ & -A_1 k_z \\ A_1 k_z & A_2 k_- & -M(\boldsymbol{k}) & 0 \\ A_2 k_+ & -A_1 k_z & 0 & -M(\boldsymbol{k}) \end{pmatrix} + \epsilon_0(\boldsymbol{k}) \tag{A.1}$$

with $k_\pm = k_x \pm i k_y$, $\epsilon_0(\boldsymbol{k}) = C + D_1 k_z^2 + D_2 k_\perp^2$ and $M(\boldsymbol{k}) = M_0 + B_1 k_z^2 + B_2 k_\perp^2$. The basis of the Hamiltonian is chosen to be $\left(\left|P_{1z}^{+\uparrow}\right\rangle, \left|P_{1z}^{+\downarrow}\right\rangle, \left|P_{2z}^{-\uparrow}\right\rangle, \left|P_{2z}^{-\downarrow}\right\rangle\right)$, with $\pm$ standing for even and odd parity and $\uparrow\downarrow$ for spin.

For a quasi-2D thin-film, we treat the direction $z$ perpendicular to the plane to be a infinite quantum well problem and project the Hamiltonian into the subspace spanned by the quantum well states of such system. To obtain an effective model, we first consider the special case with $A_1 = 0$, and the eigen-problem can be analytically solved at the $\Gamma$ point ($k_x = k_y = 0$). The eigen-wavefunctions are given by

$$\begin{aligned} |E_{n_b}, \uparrow(\downarrow)\rangle &= \sqrt{\frac{2}{d}} \sin\left(\frac{n_b \pi z}{d} + \frac{n_b \pi}{2}\right) \left|P_{1z}^{+\uparrow(\downarrow)}\right\rangle \\ |H_{n_b}, \uparrow(\downarrow)\rangle &= \sqrt{\frac{2}{d}} \sin\left(\frac{n_b \pi z}{d} + \frac{n_b \pi}{2}\right) \left|P_{2z}^{-\uparrow(\downarrow)}\right\rangle \end{aligned} \tag{A.2}$$

with the corresponding energies $E_{E_{n_b},\uparrow(\downarrow)} = C + M_0 + (D_1 + B_1)(\frac{n_b\pi}{d})^2$ and $E_{H_{n_b},\uparrow(\downarrow)} = C - M_0 + (D_1 - B_1)(\frac{n_b\pi}{d})^2$, for the integer $n_b$ as the sub-band index. Near the crossing points between the $n_b$th electron and hole sub-band, $|E_{n_b}, \uparrow(\downarrow)\rangle$ and $|H_{n_b}, \uparrow(\downarrow)\rangle$, the 3D Hamiltonian could be projected into these 4 sub-bands to obtain the low energy physics, resulting in the 4 band BHZ-like Hamiltonian

$$H_{2D}(\boldsymbol{k}) = \begin{pmatrix} \tilde{M}(\boldsymbol{k}) & 0 & 0 & A_2 k_- \\ 0 & \tilde{M}(\boldsymbol{k}) & A_2 k_+ & 0 \\ 0 & A_2 k_- & -\tilde{M}(\boldsymbol{k}) & 0 \\ A_2 k_+ & 0 & 0 & -\tilde{M}(\boldsymbol{k}) \end{pmatrix} + \tilde{\epsilon}_0(\boldsymbol{k}) \tag{A.3}$$

where $\tilde{\epsilon}(\boldsymbol{k}) = C + D_1(\frac{n_b\pi}{d})^2 + D_2 k_\perp^2$, and $\tilde{M}(\boldsymbol{k}) = M_0 + B_1(\frac{n_b\pi}{d})^2 + B_2 k_\perp^2$. This Hamiltonian has the same mathematical structure as the BHZ model which is used to describe 2D quantum spin Hall insulator. Unlike the HgTe system, the basis we consider here is composed all from spin-1/2 electrons, namely $(|E_{n_b}, \uparrow\rangle, |E_{n_b}, \downarrow\rangle, |H_{n_b}, \uparrow\rangle, |H_{n_b}, \downarrow\rangle)$ for a given sub-band index $n_b$. It should be pointed out that the electron and hole sub-bands with the same index $n_b$ carry opposite parities. Thus, we re-write the basis as $(|+\uparrow\rangle, |+\downarrow\rangle, |-\uparrow\rangle, |-\downarrow\rangle)$ in the main text for simplicity where the sign indicates the parity of the sub-bands. It is an approximation to neglect the $A_1$ term, which will couples quantum well sub-bands with different $n_b$. This approximation works well for a small thickness $d$ when all the quantum well states are well separated in energy.

### Appendix B: Hamiltonian and method used in numerical calculation

Here we show the detailed form of the tight-binding Hamiltonian (4) as

$$\epsilon_i = \begin{pmatrix} \frac{4B}{a_0^2}+M_0 & 0 & 0 & 0 \\ 0 & \frac{4B}{a_0^2}+M_0 & 0 & 0 \\ 0 & 0 & -\frac{4B}{a_0^2}-M_0 & 0 \\ 0 & 0 & 0 & -\frac{4B}{a_0^2}-M_0 \end{pmatrix} \tag{B.1}$$

$$V_{ij} = \begin{cases} \begin{pmatrix} -\frac{B}{a_0^2} & 0 & 0 & \frac{i\alpha}{2a_0} \\ 0 & -\frac{B}{a_0^2} & \frac{i\alpha}{2a_0} & 0 \\ 0 & \frac{i\alpha}{2a_0} & \frac{B}{a_0^2} & 0 \\ \frac{i\alpha}{2a_0} & 0 & 0 & \frac{B}{a_0^2} \end{pmatrix} & , j_x = i_x + 1 \\ \begin{pmatrix} -\frac{B}{a_0^2} & 0 & 0 & \frac{\alpha}{2a_0} \\ 0 & -\frac{B}{a_0^2} & -\frac{\alpha}{2a_0} & 0 \\ 0 & \frac{\alpha}{2a_0} & \frac{B}{a_0^2} & 0 \\ -\frac{\alpha}{2a_0} & 0 & 0 & \frac{B}{a_0^2} \end{pmatrix} & , j_y = i_y + 1 \\ \text{h.c.} & , j_x = i_x - 1; j_y = i_y - 1 \end{cases} \tag{B.2}$$

where $a_0$ is the lattice constant of the regularized tight-binding model. The nearest hopping for the negative $x$ ($y$) direction is the conjugate transpose of the positive one. Magnetic textures and disorders involved in this work are all on-site, and have the same shape as matrix $\epsilon_i$.

To keep the continuity of the energy bands, the Hamiltonian of the leads are chosen to be the same as the system, with the magnetization fixed along the $-\hat{z}$ direction to align with that of the skyrmion texture at large radius $\rho$. The self-energy of the leads are calculated through a quick iterative method [3].

### Appendix C: Other transport quantities

Fig. C.1 displays Hall resistance, longitudinal resistance, Hall conductance, longitudinal conductance and Hall angle for the system with parameter set (i), i.e. a QAH system in normal band regime. The Hall angle is defined as

$$\theta_{\text{Hall}} \equiv R_{xy}/R_{xx}. \tag{C.1}$$

Both $R_{xy}$ and $\theta_{\text{Hall}}$ shows an enhancement due to the increase of $R_{xx}$.

### Appendix D: Comparison between normal and inverted band

We further reveal the Hall resistance of skyrmion and anti-skyrmion case over the whole energy range (the Fermi energy varying from valence bands to the band gap to conduction bands) in Fig. D.2. For a normal insulator, the THE does not exist outside the bulk band region, as shown in Fig. D.2(a) when the Hall resistance drops to 0 for the system with parameter set (i). For the inverted region TI with parameter set (ii), as the Fermi energy moves into the gap, one should expect the Hall resistance quantized to $h/e^2$ due to the ballistic transport from the chiral edge mode, known as the Quantum Anomalous Hall effect, shown in Fig. D.2(b). In this region, the transport is dominated by the edge mode, while the THE, which is a contribution from bulk states, diminishes.

As for the model used in the main text, both the conduction and valence bands behave the same and are symmetric about the band center. The THE changes sign near the band center, similar to a previous model discussed in [4].

[1] C.-X. Liu, H. Zhang, B. Yan, X.-L. Qi, T. Frauenheim, X. Dai, Z. Fang, and S.-C. Zhang, Physical review B **81**, 041307 (2010).

[2] C.-X. Liu, X.-L. Qi, H. Zhang, X. Dai, Z. Fang, and S.-C. Zhang, Physical Review B **82**, 045122 (2010).
[3] M. L. Sancho, J. L. Sancho, and J. Rubio, Journal of Physics F: Metal Physics **14**, 1205 (1984).
[4] P. B. Ndiaye, C. A. Akosa, and A. Manchon, Physical Review B **95**, 064426 (2017).

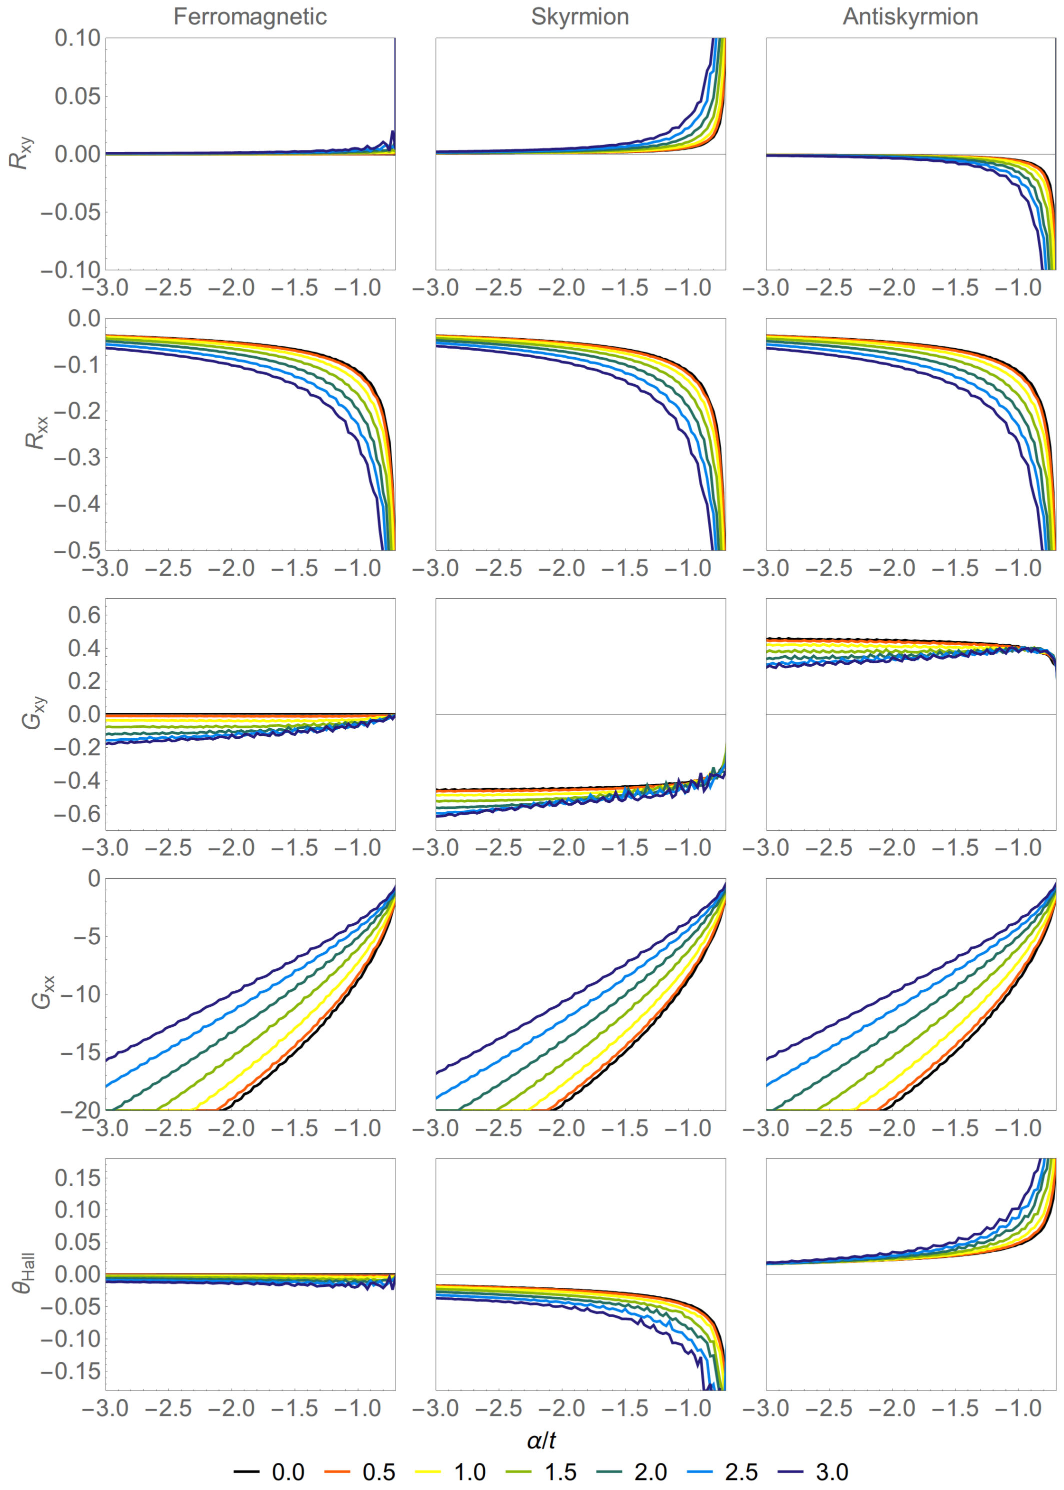


FIG. C.1. From top to bottom: Hall resistance, longitudinal resistance, Hall conductance, longitudinal conductance, Hall angle. The Hamiltonian uses parameter set (i) defined in the main text. Different color represents different SOC strength $\alpha$. Each column is for a different magnetic configuration listed on top.

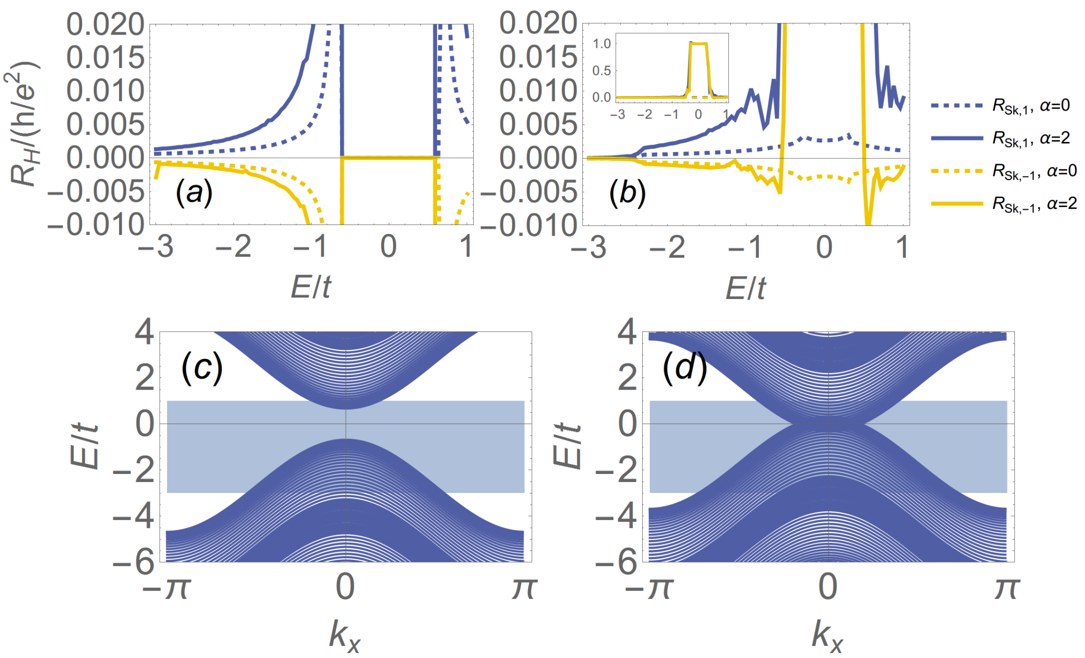


FIG. D.2. Hall resistance for (a) normal and (b) inverted band TI, for both skyrmion and antiskyrmion spin textures. Dashed lines are for SOC $\alpha = 0$ and solid lines are for SOC $\alpha = 2$ cases. For a trivial gap in (a), the Hall resistance for both spin textures reduce to zero as there are no states. For an inverted band, there is no gap for $\alpha = 0$ case thus the resistance is determined by the bulk transport. With $\alpha = 2$, the transport is determined by the edge mode and is saturated to $h/e^2$ for both spin textures. The THE in this case is also zero. (c, d) energy spectra for $\alpha = 0$, for normal band and inverted band TI, respectively, with the shades matching the Fermi energy range in the plots. Also see Fig. 1(b, c) of the main text for $\alpha = 2$ spectra.
